# Supplementary material for: Optimal Adaptive Experimental Design for Estimating Treatment Effect
Source: arXiv:2410.05552 source file (2024-11-12)
Supplement: Supplementary file 1 [file appendix.tex]

\section{Proofs}

%%%%%%%%%%%%%%%%%%%%%%%%%%%%%%%%%%%%%%%%%%%%%%%%%%%%%%%%%%%%%%%%%%%%%%%%%%%
\subsection{Proof of Lemma~\ref{prop-eqiu-existence}}
\label{proof_prop: equi-existence}
In our model, we define $\lambda_i$ as
\begin{equation*}
    \lambda_{i}=\frac{\exp (r_{i}-p_{i}-\frac{c}{\mu-\lambda})}{1+\sum_{j=1}^{n} \exp (r_{j}-p_{j}-\frac{c}{\mu-\lambda})}
\end{equation*}
Sum over $i$, we get $\lambda=\frac{\sum_{i=1}^n\exp (r_{i}-p_{i}-\frac{c}{\mu-\lambda})}{1+\sum_{j=1}^{n} \exp (r_{j}-p_{j}-\frac{c}{\mu-\lambda})}$ or $\sum_{i=1}^n \exp(r_i-p_i)= \frac{\lambda}{1-\lambda} \exp(\frac{c}{\mu-\lambda})$. Define $G(\lambda)=\frac{\lambda}{1-\lambda} \exp(\frac{c}{\mu-\lambda})$, then $G(\lambda)$ is a monotone function of $\lambda$ with $G(0)=0$ and $G(\min\{1,\mu\})=\infty$, we know that there exists a unique solution.
\QEDA

%%%%%%%%%%%%%%%%%%%%%%%%%%%%%%%%%%%%%%%%%%%%%%%%%%%%%%%%%%%%%%%%%%%%%%%%%%%%%%

\subsection{Proof of Proposition~\ref{prop-optpric}}
\label{proof_prop: optpric}
Note that the pricing optimization can be written as
\begin{equation}
    \begin{aligned}
\max \quad& R (\boldsymbol{\lambda}, \lambda)=\sum_{i=1}^n \lambda_i\left(r_i-\log \lambda_i\right)+\log \left(1-\lambda\right) \lambda-c\frac{\lambda}{\mu-\lambda} \\
\text { s.t. } & \sum_{i=1}^n \lambda_i=\lambda, \\
& \lambda \leq 1, \\
& \sum_{i=1}^n \lambda_i \leq \mu\\
& \lambda_i \ge 0
\end{aligned} 
\end{equation}
Using KKT condition, the optimal $\boldsymbol{\lambda}^{*}$ and $\lambda^{*}$ should satisfy
\begin{equation}
\begin{aligned}
\frac{\partial R}{\partial \lambda_i}(\boldsymbol{\lambda}, \lambda)-\eta_1- \eta_3+\kappa_i & =0, i=1, \ldots, n ; \\
\frac{\partial R}{\partial \lambda}(\boldsymbol{\lambda}, \lambda)+\eta_1-\eta_2 & =0 ; \\
\sum_{i=1}^n \lambda_i-\lambda & =0 ; \\
\eta_2(\lambda-1) & =0 ;\\
\eta_3\left(\sum_{i=1}^n \lambda_i -\mu\right) & =0 ; \\
\kappa_i \lambda_i & =0, i=1, \ldots, n ; \\
\eta_2, \eta_3 & \geq 0 ; \\
\kappa_i & \geq 0, i=1, \ldots, n,
\end{aligned}
\end{equation}
where $\eta_1, \eta_2, \eta_3$ are the Lagrange multipliers for constraints $\sum_{i=1}^n \lambda_i=\lambda, \lambda \leq 1, \sum_{i=1}^n \lambda_i \leq \mu$, respectively, and $\kappa_i$ the Lagrange multiplier for the constraint $\lambda_i \geq 0, i=1, \ldots, n$. It is also easy to verify the optimal solution $\lambda^*$ and $\lambda^*$ satisfy $\sum_{i=1}^n<1, \sum_{i=1}^n \lambda_i^* <\mu1$ and $\lambda_i^*>0$. Thus, we have $\eta_2^*=\eta_3^*=0$ and $\kappa_i^*=0$ for $i=1, \ldots, n$. Then, from $(7)$, we have $\frac{\partial R}{\partial \lambda_i}\left(\lambda^*, \lambda^*\right)=\eta_1^*$ for $i=1, \ldots, n$. That is,
\begin{equation}
    r_i-\log \lambda_i^*-1-c\frac{\lambda}{\mu-\lambda}=\eta_1^*, i=1, \ldots, n
\end{equation}
which tells us that 
$$
r_i-\log \lambda_i^*=r_j-\log \lambda_j^* .
$$
for any $i,j \in {1 ,\cdots, n}$.
This implies $\lambda_i^* / \lambda_j^*=e^{r_i} / e^{r_j}$. Since $\sum_{i=1}^n \lambda_i^*=\lambda^*$, we have
$$
\lambda_i^*=\frac{e^{r_i}}{\sum_{j=1}^n e^{r_j}} \lambda^* .
$$
Again, by KKT condition, $\lambda_i^*$ and $\lambda^*$ satisfy $\frac{\partial R}{\partial \lambda_i}(\boldsymbol{\lambda}, \lambda)-\eta_1=0$ and $\frac{\partial R }{\partial \lambda}(\boldsymbol{\lambda}, \lambda)+\eta_1=0$, which imply $\frac{\partial R}{\partial \lambda_i}\left(\lambda^*, \lambda^*\right)+\frac{\partial R}{\partial \lambda}\left(\lambda^*, \lambda^*\right)=0$, and so
$$
\left(r_i-\log \lambda_i^*\right)-1+\log \left(1-\lambda^*\right)-\frac{\lambda^*}{1-\lambda^*}-c \frac{\mu}{\left(\mu-\lambda^*\right)^2}=0 .
$$
Plugging in $\lambda_i^*=\frac{e^{r_i}}{\sum_{j=1}^n e^{r_j}} \lambda^*$ gives
$$
\log \sum_{j=1}^n e^{r_j}-1-\log \lambda^*+\log \left(1-\lambda^*\right)-\frac{\lambda^*}{1-\lambda^*}-c \frac{\mu}{\left(\mu-\lambda^*\right)^2}=0,
$$
which is equivalent to (\ref{prop-optpric:optimal-lambda}). Defining $F(\lambda):=\log \sum_{j=1}^n e^{r_j}-1-\log \lambda+\log \left(1-\lambda\right)-\frac{\lambda}{1-\lambda}-c \frac{\mu}{(\mu-\lambda)^2}, \lambda^*$ solves $F(\lambda)=0$. Since
$$
F^{\prime}(\lambda)=-\frac{1}{\lambda}-\frac{\lambda}{1-\lambda}-\frac{1}{(1-\lambda)^2}-2 c \frac{\mu}{(\mu-\lambda)^3}<0,
$$
$\lim _{\lambda \rightarrow 0} F(\lambda)=\infty$ and $\lim _{\lambda \rightarrow \min \{1, \mu\}} F(\lambda)=-\infty$, it follows that there exits an unique solution to $F(\lambda)=0$ in $(0, \min \{\Lambda, \mu\})$. Finally,
$$
p_i^*=p\left(\lambda_i^*\right)=\left(r_i-\log \lambda_i^*\right)+\log \left(1-\lambda^*\right)-c \frac{1}{\mu-\lambda^*}=\log \sum_{j=1}^n e^{r_j}-\log \lambda^*+\log \left(1-\lambda^*\right)-c \frac{1}{\mu-\lambda^*},
$$
which is equivalent to (\ref{prop-optpric:opt-price}).
\QEDA

%%%%%%%%%%%%%%%%%%%%%%%%%%%%%%%%%%%%%%%%%%%%%%%%%%%%%%%%%%%%%%%%%%%%%%%%%%%%%%

\subsection{Proof of Lemma~\ref{prop-optpric:structure}}
\label{proof_prop-optpirc: structure}
 Part 1. Let $a=\log \sum_{j=1}^n e^{r_j}-1$ and
$$
F(\lambda, \mu,  c)=a-\log \frac{\lambda}{1-\lambda}-\frac{\lambda}{1-\lambda}-c \frac{\mu}{(\mu-\lambda)^2} .
$$
Then $\lambda^*$ is the unique solution to $F(\lambda, \mu, c)=0$. Since
$$
\begin{aligned}
\frac{\partial F}{\partial \lambda}=-\frac{1}{\lambda}-\frac{\lambda}{1-\lambda}-\frac{1}{(1-\lambda)^2}-\frac{2 c \mu}{(\mu-\lambda)^3}<0, \frac{\partial F}{\partial \mu}=\frac{c(\mu+\lambda)}{(\mu-\lambda)^3}>0 \\
\end{aligned}
$$
by implicit function theorem,
$$
\frac{d \lambda}{d \mu}=-\frac{\partial F}{\partial \mu} / \frac{\partial F}{\partial \lambda}=\frac{c \frac{\mu+\lambda}{(\mu-\lambda)^3}}{\frac{1}{\lambda}+\frac{\lambda}{1-\lambda}+\frac{1}{(1-\lambda)^2}+2 c \frac{\mu}{(\mu-\lambda)^3}}<\frac{c \frac{\mu+\lambda}{(\mu-\lambda)^3}}{2 c \frac{\mu}{(\mu-\lambda)^3}}=\frac{\mu+\lambda}{2 \mu}<1,
$$
Clearly $\frac{d \lambda}{d \mu}>0$ and $\frac{d \lambda}{d c}<0 $.

 Part 2(i). Solving $F(\lambda, \mu, , c)=0$ gives the relation between $\lambda^*$ and $\mu$, and we write $\lambda^*(\mu)$ to denote the dependence of $\lambda^*$ on $\mu$. By Part $1, \lambda^*(\mu)$ is increasing in $\mu$ with an increasing rate less than 1. Hence, the inverse function $\mu\left(\lambda^*\right)$ is also increasing in $\lambda^*$ with an increasing rate larger than 1. To study the impact of $\mu$ on $p_i^*$, it suffices to examine the impact of $\lambda^*$ on $p_i^*$ for fixed $c$.
Define $K\left(\lambda^*\right):=\frac{1}{\mu\left(\lambda^*\right)-\lambda^*}$. Since $F\left(\lambda^*, \mu,  c\right)=0$, we have
$$
a-\log \frac{\lambda^*}{1-\lambda^*}-\frac{\lambda^*}{1-\lambda^*}-c K\left(\lambda^*\right)-c \lambda K^* 2\left(\lambda^*\right)=0 .
$$
Differentiating with respect to $\lambda^*$ gives
$$
-\frac{1}{\lambda^*\left(1-\lambda^*\right)}-\frac{1}{\left(1-\lambda^*\right)^2}-c\left(1+2 \lambda^* K\left(\lambda^*\right)\right) K^{\prime}\left(\lambda^*\right)-c K^2\left(\lambda^*\right)=0,
$$
which implies
$$
K^{\prime}\left(\lambda^*\right)=-\frac{\frac{1}{\lambda^*\left(1-\lambda^*\right)}+\frac{1}{\left(1-\lambda^*\right)^2}+c K^2\left(\lambda^*\right)}{c\left(1+2 \lambda^* K\left(\lambda^*\right)\right)} .
$$
By $(9), p_i^*=p_i\left(\lambda^*\right)=a+1-\log \frac{\lambda^*}{1-\lambda^*}-c K\left(\lambda^*\right)$, and so
$$
\begin{aligned}
p_i^{\prime}\left(\lambda^*\right) & =-\frac{1}{\lambda^*\left(1-\lambda^*\right)}-c K^{\prime}\left(\lambda^*\right) \\
& =-\frac{1}{\lambda^*\left(1-\lambda^*\right)}+\frac{\frac{1}{\lambda^*\left(1^* \lambda^*\right)}+\frac{1}{\left(1-\lambda^*\right)^2}+c K^2\left(\lambda^*\right)}{1+2 \lambda^* K\left(\lambda^*\right)} \\
& =-\frac{2 \lambda^* K\left(\lambda^*\right)}{1+2 \lambda^* K\left(\lambda^*\right)} \frac{1}{\lambda^*\left(1-\lambda^*\right)}+\frac{1}{1+2 \lambda^* K\left(\lambda^*\right)} \frac{1}{\left(1-\lambda^*\right)^2}+\frac{1}{1+2 \lambda^* K\left(\lambda^*\right)} c K^2\left(\lambda^*\right) \\
& =-\frac{2 \lambda^*}{\mu\left(\lambda^*\right)+\lambda^*} \frac{1}{\lambda^*\left(1-\lambda^*\right)}+\frac{\mu\left(\lambda^*\right)-\lambda^*}{\mu\left(\lambda^*\right)+\lambda^*} \frac{1}{\left(1-\lambda^*\right)^2}+\frac{\mu\left(\lambda^*\right)-\lambda^*}{\mu\left(\lambda^*\right)+\lambda^*} c \frac{1}{\left(\mu\left(\lambda^*\right)-\lambda^*\right)^2} \\
& =\frac{1}{\left(\mu\left(\lambda^*\right)+\lambda^*\right)\left(\mu\left(\lambda^*\right)-\lambda^*\right)}\left[-2 1 \frac{\mu\left(\lambda^*\right)-\lambda^*}{1-\lambda^*}+1\left(\frac{\mu\left(\lambda^*\right)-\lambda^*}{1-\lambda^*}\right)^2+c\right] .
\end{aligned}
$$
Clearly, the sign of $p_i^{\prime}\left(\lambda^*\right)$ is determined by $f_1\left(\lambda^*\right):=-2  \frac{\mu\left(\lambda^*\right)-\lambda^*}{1-\lambda^*}+\left(\frac{\mu\left(\lambda^*\right)-\lambda^*}{1-\lambda^*}\right)^2+c$.
When $c \geq 1, f_1\left(\lambda^*\right)=\left(\frac{\mu\left(\lambda^*\right)-\lambda^*}{1-\lambda^*}-1\right)^2+c-1\geq 0$. Thus, $p_i^{\prime}\left(\lambda^*\right) \geq 0$ and $p_i^*$ is increasing in $\lambda^*$ and thus increasing in $\mu$.
When $c<1, f_1\left(\lambda^*\right) \geq 0$ if $\frac{\mu\left(\lambda^*\right)-\lambda^*}{1-\lambda^*} \geq 1+\sqrt{1-c}$ or $\frac{\mu\left(\lambda^*\right)-\lambda^*}{1-\lambda^*} \leq 1-\sqrt{1-c}$, and $f_1\left(\lambda^*\right) \leq 0$ if $1-$ $\sqrt{1-c} \leq \frac{\mu\left(\lambda^*\right)-\lambda^*}{1-\lambda^*} \leq 1+\sqrt{1-c}$. Note also that $\frac{\mu\left(\lambda^*\right)-\lambda^*}{1-\lambda^*}$ is increasing in $\lambda^*$ since the numerator increases with $\lambda^*$ (see Part 1 ) and the denominator decreases with $\lambda^*$. Let $\underline{\lambda}_1$ be the solution to
$\frac{\mu\left(\lambda^*\right)-\lambda^*}{1-\lambda^*}=1-\sqrt{1-c}$ and $\bar{\lambda}_1$ be the solution to $\frac{\mu\left(\lambda^*\right)-\lambda^*}{1-\lambda^*}=1+\sqrt{1-c}$ (one can show $\underline{\lambda}_1$ and $\bar{\lambda}_1$ always exist and are unique because the range of $\frac{\mu\left(\lambda^*\right)-\lambda^*}{1-\lambda^*}$ is $(0, \infty)$.) Hence, when $0 \leq \lambda^* \leq \underline{\lambda}_1$ or $\lambda^* \geq \bar{\lambda}_1$, it holds that $f_1\left(\lambda^*\right) \geq 0$ and $p_i^{\prime}\left(\lambda^*\right) \geq 0$. When $\underline{\lambda}_1 \leq \lambda^* \leq \bar{\lambda}_1$, it holds that $f_1\left(\lambda^*\right) \leq 0$ and
8
$p_i^{\prime}\left(\lambda^*\right) \leq 0$. Since $\mu\left(\lambda^*\right)$ is increasing in $\lambda^*$, it follows tha $p_i^*$ is increasing in $\mu$ for $0 \leq \mu \leq \underline{\mu}:=\mu\left(\underline{\lambda}_1\right)$ and $\mu \geq \bar{\mu}:=\mu\left(\bar{\lambda}_1\right)$, and decreasing in $\mu$ for $\underline{\mu} \leq \mu \leq \bar{\mu}$.

Part 2(ii). To study the impact of $c$ on $p_i^*$, it suffices to examine the impact of $\lambda^*$ on $p_i^*$ for fixed $\mu$. Since $F\left(\lambda^*, \mu,  c\right)=0$, we have
$$
c\left(\lambda^*\right)=\frac{a-\log \frac{\lambda^*}{1-\lambda^*}-\frac{\lambda^*}{1-\lambda^*}}{\mu /\left(\mu-\lambda^*\right)^2}
$$
which is decreasing in $\lambda^*$. Then,
$$
\begin{aligned}
p_i^*=p_i\left(\lambda^*\right)=1+\frac{\lambda^*}{1-\lambda^*}+c \frac{\lambda^*}{\left(\mu-\lambda^*\right)} & =1+\frac{\lambda^*}{1-\lambda^*}+\frac{a-\log \frac{\lambda^*}{1-\lambda^*}-\frac{\lambda^*}{1-\lambda^*}}{\mu /\left(\mu-\lambda^*\right)^2} \frac{\lambda^*}{\left(\mu-\lambda^*\right)} \\
& =1+\frac{\lambda^*}{1-\lambda^*}+\frac{\lambda^*}{\mu}\left[a-\log \frac{\lambda^*}{1-\lambda^*}-\frac{\lambda^*}{1-\lambda^*}\right],
\end{aligned}
$$
and so
$$
p_i^{\prime}\left(\lambda^*\right)=\left(1-\frac{1}{\mu}\right) \frac{1}{\left(1-\lambda^*\right)^2}+\frac{1}{\mu}\left[a-\log \frac{\lambda^*}{1-\lambda^*}-\frac{\lambda^*}{1-\lambda^*}\right] \text {. }
$$
It is easy to verify $a-\log \frac{\lambda^*}{1-\lambda^*}-\frac{\lambda^*}{1-\lambda^*}>0$. When $\mu \geq 1, p_i^{\prime}\left(\lambda^*\right)>0$ and $p_i^*$ is increasing in $\lambda^*$. Since $c$ is decreasing in $\lambda^*$, it follows that $p_i^*$ is decreasing in $c$.

When $\mu<1, p_i^{\prime \prime}\left(\lambda^*\right)=\left(1-\frac{1}{\mu}\right) \frac{2 }{\left(1-\lambda^*\right)^3}+\frac{1}{\mu}\left[-\frac{1}{\lambda^*}\left(\frac{1}{\left(1-\lambda^*\right)^2}\right)\right]<0$. Hence, $p_i^{\prime}\left(\lambda^*\right)$ is decreasing in $\lambda^*$. When $\log \left(\sum_j e^{r_j}\right)-\log \frac{\mu}{\Lambda-\mu}-\frac{1+\mu}{1-\mu} \geq 1$, one can verify $p_i^{\prime}\left(\lambda^*\right) \geq 0$ for $\lambda^*$ close to $\mu$, in which case, $p_i^{\prime}\left(\lambda^*\right)>0$ for all $\lambda^*<\mu$. So $p_i^*$ is increasing in $\lambda^*$ and thus decreasing in $c$. Otherwise, if $\log \left(\sum_j e^{r_j}\right)-\log \frac{\mu}{1-\mu}-\frac{1+\mu}{1-\mu}<1$, then there exists a unique solution to $p_i^{\prime}\left(\lambda^*\right)=0$ denoted by $\lambda_3$. When $\lambda^* \leq \lambda_3$, it holds that $p_i^{\prime}\left(\lambda^*\right) \geq 0$. When $\lambda^* \geq \lambda_3$, it holds that $p_i^{\prime}\left(\lambda^*\right) \leq 0$. Since $c$ is decreasing in $\lambda^*$, it follows that $p_i$ is decreasing in $c$ for $c \geq c_3:=c\left(\lambda_3\right)$ and increasing in $c$ for $c \leq c_3$.

Part 3. Similar to the proof of Part 2, to study the impacts of $\mu$ and $c$ on the optimal profit $R^*$, it suffices to write each component as a function of $\lambda^*$ and examine its impact while fixing the other two components.

When  $c$ is fixed, we write $\mu$ as a function of $\lambda^*$ and plug it into $^*$. Then $\left.R^*=R^* (\lambda^*\right)=$ $p_i\left(\lambda^*\right) \lambda^*$, and so
$$
\begin{aligned}
R^{\prime}\left(\lambda^*\right) & =p_i^{\prime}\left(\lambda^*\right) \lambda^*+p_i\left(\lambda^*\right) \\
& =\left[-\frac{2 \lambda^* K\left(\lambda^*\right)}{1+2 \lambda^* K\left(\lambda^*\right)} \frac{1}{\lambda^*\left(1-\lambda^*\right)}+\frac{1}{1+2 \lambda^* K\left(\lambda^*\right)} \frac{1}{\left(1-\lambda^*\right)^2}+\frac{1}{1+2 \lambda^* K\left(\lambda^*\right)} c K^2\left(\lambda^*\right)\right] \lambda^* \\
& \quad+1+\frac{1}{1-\lambda^*}+c \lambda^* K^2\left(\lambda^*\right) \\
& =1+\frac{1}{1+2 \lambda^* K\left(\lambda^*\right)} \frac{1}{1-\lambda^*}+\frac{\lambda^*}{1+2 \lambda^* K\left(\lambda^*\right)} \frac{1}{\left(1-\lambda^*\right)^2}+c \lambda^* K^2\left(\lambda^*\right)\left[1+\frac{1}{1+2 \lambda^* K\left(\lambda^*\right)}\right] \\
& >0 .
\end{aligned}
$$
Since $\mu\left(\lambda^*\right)$ is increasing in $\lambda^*, R^*$ is increasing in $\mu$.
When $\mu$ and $c$ are fixed, we write $\Lambda$ as a function of $\lambda^*$ and plug it into $R^*$. Then,
$$
R^{\prime}\left(\lambda^*\right)=p_i^{\prime}\left(\lambda^*\right) \lambda^*+p_i\left(\lambda^*\right)
$$
When $\mu$ is fixed, we write $c$ as a function of $\lambda^*$ and plug it into $R^*$. Then,
$$
R^{\prime}\left(\lambda^*\right)=p_i^{\prime}\left(\lambda^*\right) \lambda^*+p_i\left(\lambda^*\right)
$$
$$
\begin{aligned}
& =\left[\left(1-\frac{1}{\mu}\right) \frac{1}{\left(1-\lambda^*\right)^2}+\frac{1}{\mu}\left(a-\log \frac{\lambda^*}{1-\lambda^*}-\frac{\lambda^*}{1-\lambda^*}\right)\right] \lambda^*+1+\frac{\lambda^*}{1-\lambda^*}+\frac{\lambda^*}{\mu}\left[a-\log \frac{\lambda^*}{1-\lambda^*}-\frac{\lambda^*}{1-\lambda^*}\right] \\
& \geq\left[\left(1-\frac{1}{\lambda^*}\right) \frac{1}{\left(1-\lambda^*\right)^2}+\frac{1}{\mu}\left(a-\log \frac{\lambda^*}{1-\lambda^*}-\frac{\lambda^*}{1-\lambda^*}\right)\right] \lambda^*+1+\frac{\lambda^*}{1-\lambda^*}+\frac{\lambda^*}{\mu}\left[a-\log \frac{\lambda^*}{1-\lambda^*}-\frac{\lambda^*}{1-\lambda^*}\right] \\
& =2 \frac{\lambda^*}{1-\lambda^*}+\frac{\lambda^*}{\mu}\left[a-\log \frac{\lambda^*}{1-\lambda^*}-\frac{\lambda^*}{1-\lambda^*}\right] \\
& >0 .
\end{aligned}
$$
Since $c\left(\lambda^*\right)$ is decreasing in $\lambda^*, R^*$ is increasing in $c$.
\QEDA

%%%%%%%%%%%%%%%%%%%%%%%%%%%%%%%%%%%%%%%%%%%%%%%%%%%%%%%%%%%%%%%%%%%%%%%%%%%%%%%%%%%

\subsection{Proof of Theorem~\ref{thm-assortment-hardness}}
\label{proof_thm: assortment-hardness}
\textbf{NP-Hardness} In order to prove that the assortment optimization problem is NP-hard, we will show that $T$-feasibility problem is NP-complete, which is defined as
\begin{definition}\label{T-feasibility}
   For any given product set $\{(r_i,p_i)\}_{i=1}^n$, c, $\mu$ and any $T$, whether there exists an assortment $S$ such that the revenue $R(S) \ge T$? 
\end{definition}
If there is no polynomial time algorithm that can solve T-feasibility problem, the feasibility problem for assortment is NP-complete. We will prove that feasibility problem for assortment (\ref{equ-assortment}) is NP-complete with reduction from \textit{Partition problem}(\textbf{ref}), which is well-known to be NP-complete. 
\begin{definition}
    Given a set of n number $\omega_i$ such that $\sum_{i=1}^n \omega_i=2$, whether there exists a subset $S$ such that $\sum_{i \in S} \omega_i=1$.
\end{definition}

For any instance $I$ of \textit{Partition Problem} $\{\omega_i\}_{i=1}^n$, we will construct an instance of assortment optimization problem and show that they are equivalent.
Consider $n+1$ products, with the first n product having utility $\omega_i=\exp(r_i-p_i)$ as the set $\{\omega_i\}_{i=1}^n$ in Instance $I$ (Note that we can always modify $r_i$ to make it satisfied,) and same price $p_1$. And product $n+1$ has utility $\omega_{n+1}$ and $p_2>p_1$. 
Note that as long as $p_2>p_1$, including product n+1 will always be beneficial, we choose T such that we must choose product $n+1$.. 
Denote $N={1,2,\cdots,n}$, then $T$ need to satisfy that 
$T>np_1 \cdot \lambda_N$. The revenue function now will be a function of the sum of utility of first n products.
$$
F(\omega)=\left(p_{1} \omega+p_{2} \omega_{n+1}\right) \frac{\lambda}{\omega+\omega_{n+1}}
$$
So now we need to design a function such that the only maximum value  is attained at $\omega=1$.
Note that $\lambda$ and $\omega$ has a one-to-one map and $\omega$  is increasing with $\lambda$. We denote as $\omega=h(\lambda)$
So in the following we denote $G(\lambda)=F(h(\lambda))$ as a function of $\lambda$ with a unique maximizer $h^{-1}(1)$. 
\begin{equation}
    \begin{aligned}
        G(\lambda)&=\left.p_{1}\left(\frac{\lambda}{1-\lambda} \exp \left(\frac{c}{\mu-\lambda}\right)-\omega_{n+1}\right)+p_{2} \omega_{n+1}\right) \cdot(1-\lambda) \exp \left(-\frac{c}{\mu-\lambda}\right)\\
&=p_{1} \cdot \lambda+\left(p_{2}-p_{1}\right) w_{n+1} \cdot(1-\lambda) \exp \left(-\frac{c}{\mu-\lambda}\right)\\   
       G^{'}(x)&= p_{1}-\left(c \cdot \frac{(1-x)}{(\mu-x)^{2}}+1\right) \exp \left(-\frac{c}{\mu-x}\right) \omega_{n+1}\left(p_{2}-p_{1}\right)
    \end{aligned}
\end{equation}
If $G^{'}(x)$, or $-\left(c \cdot \frac{(1-x)}{(\mu-x)^{2}}+1\right) \exp \left(-\frac{c}{\mu-x}\right) \omega_{n+1}\left(p_{2}-p_{1}\right)$ is decreasing in
 $x \in [0,\lambda_{max}]$, and $G^{'}(h^{-1}(1))=0$, we know that $\omega=1$ is the unique maximizer of $F$ and we can set $T=F(1)$ to show that T-feasibility problem in definition (\ref{T-feasibility}) is equivalent to \textit{Partition Problem} instance $I$.
 So the feasibility set is
 \begin{equation}\label{equ-feasibility-set}
 \begin{cases}
     p_{1}=\left(c \cdot \frac{1-h^{-1}(1)}{(\mu-h^{-1}(1))^{2}}+1\right) \exp \left(-\frac{c}{\mu-h^{-1}(1)}\right) \omega_{n+1}\left(p_{2}-p_{1}\right)\\
     \frac{2(1-\mu) \mu-c }{2\left(1-\mu-\frac{c}{2}\right)}\ge\lambda_{\max }\\
      w_{n+1}+2=\frac{\lambda_{\max }}{1-\lambda_{\max }} \cdot \exp \left(\frac{c}{\mu-\lambda_{\max }}\right) 
 \end{cases} 
\end{equation}
If we find feasible solution of $c$, $\mu$,  $p_1$, $p_2$, $\omega_{n+1}$ for (\ref{equ-feasibility-set}), then $h^{-1}(1)$ is the only maximizer of $G(\lambda)$, where $h^{-1}(1)$ represents the solution of
$$w_{n+1}+1=\frac{\lambda}{1-\lambda} \cdot \exp \left(\frac{c}{\mu-\lambda}\right)$$

Set $\lambda_{max}=0.9$, $\mu=0.95$, $c=0.05$, $\omega_{n+1}=9e-2$. 
Then we can get $h^{-1}(1)\approx 0.899$. Take it back to the first equation in (\ref{equ-feasibility-set}), we can set $p_1=1$, $p_2\approx 1.04$ and one can check that the feasibility of (\ref{equ-feasibility-set}) is satisfied. Thus we have proved that T-feasibility problem for assortment is NP-complete.

\noindent{\textbf{Revenue-order Assortment}}
As the second part of theorem \ref{thm-assortment-hardness}, we will prove that if and only if one of the following condition is satisfied: (a). $\mu \ge 1$ (b). $c \ge 2\mu(1-\mu)$ (we assume that $c>0$, otherwise it's trivial), revenue-order assortment is optimal for any possible product set $(r_i,p_i)$, $i=1,\cdots,n$.
In order to prove the condition is sufficient and necessary, we need the following theorem from \cite{talluri2004revenue}:
\begin{theorem}\label{thm-revenue-order-optimal}
       A choice model has the nested-by-fare-order property iff i) The probability of purchase, $Q(S)$, is increasing, and ii) for every incomplete set $T$ there exist a set of convex weights $\alpha_{j}, j=1, \ldots, n$, satisfying $\alpha_{j} \geq 0$ and $\sum_{j=1}^{n} \alpha_{j}=1$, such that the probabilities defined by
$$
\bar{P}_{j}(\alpha)=\sum_{k=1}^{n} \alpha_{k} P_{j}\left(S_{k}\right), \quad j=1, \ldots, n
$$
satisfy
$$
\sum_{j=1}^{i} \bar{P}_{j}(\alpha) \geq \sum_{j=1}^{i} P_{j}(T), \quad i=1, \ldots, n-1
$$
and
$$
\sum_{j=1}^{n} \bar{P}_{j}(\alpha)=\sum_{j=1}^{n} P_{j}(T)
$$
\end{theorem}
\noindent{\textbf{Sufficient}}
In this part, we assume that at least one of (a). $\mu \ge 1$ (b). $c \ge 2\mu(1-\mu)$ is satisfied, so we need to show that the condition in theorem \ref{thm-revenue-order-optimal} is satisfied.

The revenue function can be written as $\sum_{j \in S} \lambda_j*p_j$ or
    \begin{equation}
        \begin{aligned}
            \sum _{i \in S}\frac {p_i*exp(r_i-p_i-c/(\mu-\lambda)} {1+\sum_{j=1}^n exp(r_i-p_i-c/(\mu-\lambda))}           
        \end{aligned}
    \end{equation}
    We multiply $\exp(c/(\mu-\lambda))$ to  make other terms as constant. So equivalently
    \begin{equation}
        \begin{aligned}
            \sum _{i \in S}\frac {p_i*exp(r_i-p_i)} {exp(c/(\mu-\lambda))+\sum_{j=1}^n exp(r_i-p_i)}          
        \end{aligned}
    \end{equation}
 To be brief, we will denote  $\exp(r_i-p_i)$ as $w_i$.
    In the following, we will denote $\sum_{i \in S} w_i$ as $\mathcal{W}$.
    Recall that $\lambda$ is decided by
    \begin{equation}\label{equ-lambda}
        \begin{aligned}
            \mathcal{W}=\lambda/(1-\lambda)*\exp(c/(\mu-\lambda))       
        \end{aligned}
    \end{equation}
    It's easy to find that $\lambda$ is increasing with $\mathcal{W}$ and vice versa.  

    So in the following we will check each condition in theorem \ref{thm-revenue-order-optimal}.
    First of all, it's clear from equation (\ref{equ-lambda}) that $Q(S)=\sum_{i \in S}\lambda_i=\lambda$
    is increasing with S.
    To show the second set of condition in Theorem 2,
    let T be an incomplete set and 
    define the index $k$ by
    \begin{equation}
        \begin{aligned}
            \sum _{i=1}^{k} w_i \le \ \sum _{i \in T} w_i <\sum _{i=1}^{k+1} w_i              
        \end{aligned}
    \end{equation}
    Note that $k$ is less than the largest index in T; that is, $max{\{j : j \in T\}} > k$. 
    Denote $S_k=\{1,\cdots, k\}$ and each $\lambda$ in $S_k$, $S_{k+1}$ ,$T$ as $\lambda_{k}$, $\lambda_{k+1}$
    and $\lambda_T$, so $\lambda_{k}\le \lambda_T < \lambda_{k+1}$
    Next, define $\alpha$ by
    \begin{equation}\label{equ-convex-weight}
        \begin{aligned}
            \alpha \frac{\sum_{i=1}^k w_i} {exp(c/(\mu-\lambda_k))+\sum_{i=1}^k w_i} + (1-\alpha)\frac{\sum_{i=1}^{k+1} w_i} {exp(c/(\mu-\lambda_{k+1}))+\sum_{i=1}^{k+1} w_i}=\frac{\sum_{i \in T} w_i} {exp(c/(\mu-\lambda_T))+\sum_{i \in T} w_i}              
        \end{aligned}
    \end{equation}
    Here we propose a lemma:
    under the condition we assume, we have
\begin{lemma}\label{lem-convexity}
  \begin{equation}
        \begin{aligned}
            \alpha \frac{1}{\sum_{i \in A_k}w_i+\exp(c/(\mu-\lambda_k))} +(1-\alpha) \frac{1}{\sum_{i \in A_{k+1}}a_i+\exp(c/(\mu-\lambda_{k+1}))} \ge \frac{1}{\sum_{i \in T} a_i+\exp(c/(\mu-\lambda_T))  }                
        \end{aligned}
    \end{equation}
\end{lemma}

    We will prove this lemma at the final part.
    Now assuming lemma \ref{lem-convexity},define the convex weights
    $\alpha_j=\alpha$ when $j=k$, $\alpha_j=1-\alpha$ when $j=k+1$,
    and in other cases set $\alpha_j=0$.
    Using these weights and MNL probabilities, we know that for $j \le k$
    \begin{equation}
        \begin{aligned}
            \hat{P}_j(\alpha)=& 
            \alpha P_j(S_k)+(1-\alpha) P_j(S_{k+1}) \\
            =&w_j* (\alpha *\frac{1}{\sum_{i \in S_k}w_i+\exp(c/(\mu-\lambda_k))} +(1-\alpha) *\frac{1}{\sum_{i \in S_{k+1}}w_i+\exp(c/(\mu-\lambda_{k+1}))} )\\
            \ge& w_j* \frac{1}{\sum_{i \in T} w_i+\exp(c/(\mu-\lambda_T))}   \\ 
            \ge& P_j(T)
        \end{aligned}
    \end{equation}
    So for $j \le k$, we have 
    \begin{equation}
        \begin{aligned}
            \sum _{i=1}^j \hat{P}_j(\alpha) \ge \sum _{i=1}^j P_j(T)
        \end{aligned}
    \end{equation}
    as required by Theorem 2.
    
    For $j > k$
    \begin{equation}
        \begin{aligned}
            \sum _{i=1}^j \hat{P}_j(\alpha) =& \alpha *\frac{\sum_{i \in S_k}w_i}{\sum_{i \in S_k}w_i+\exp(c/(\mu-\lambda_k))}           +(1-\alpha) *\frac{\sum_{i \in S_{k+1}}w_i}{\sum_{i \in S_{k+1}}w_i+\exp(c/(\mu-\lambda_{k+1}))} \\
            =& \frac{\sum_{i \in T}w_i}{\sum_{i \in T} w_i+\exp(c/(\mu-\lambda_T))}\\
            \ge& \sum _{i=1}^j P_j(T)          
        \end{aligned}
    \end{equation}
    where the second equation comes from equation (\ref{equ-convex-weight}).
    And for $j=n$, by equation (\ref{equ-convex-weight}), we get the equality.
   So far we have proved the condition in theorem \ref{thm-revenue-order-optimal}, so it's a
    nested by fare structure.
    
    At last, we will prove lemma \ref{lem-convexity}.Use equation (\ref{equ-lambda}), lemma \ref{lem-convexity} becomes
    \begin{equation}
        \begin{aligned}
            &\alpha \frac {1}{\lambda_k/(1-\lambda_k)*\exp(c/(\mu-\lambda_k))+\exp(c/(\mu-\lambda_k))} \\
            +&(1-\alpha)  \frac {1}{\lambda_{k+1}/(1-\lambda_{k+1})*\exp(c/(\mu-\lambda_{k+1}))+\exp(c/(\mu-\lambda_{k+1}))} \\
            \ge&\frac {1}{\lambda_T/(1-\lambda_T)*\exp(c/(\mu-\lambda_T))+\exp(c/(\mu-\lambda_T))}    
        \end{aligned}
    \end{equation}
    And $\alpha$ is defined as $\alpha \lambda_k+(1-\alpha)\lambda_{k+1}=\lambda_T$,
    so this is equivalent to the convexity of function
    \begin{equation}\label{equ-convex-function}
        \begin{aligned}
            &\frac{1}{\lambda/(1-\lambda)*\exp(c/(\mu-\lambda))+\exp(c/(\mu-\lambda))}\\
            &=(1-\lambda)*\exp(-c/(\mu-\lambda))
        \end{aligned}
    \end{equation}
    And the second derivative of this function is
    \begin{equation}
        \begin{aligned}
            c*\exp(-c/(\mu-x))*\frac {c(1-x)-2(1-\mu)(\mu-x)}{(\mu-x)^4}
        \end{aligned}
    \end{equation}
    Thus when $\mu\ge 1$ or $c\ge2\mu(1-\mu)$, by checking $x=0$ and $x=\min\{\mu,1\}$
    we prove that the function is convex. So the sufficient part is completed.
    
\noindent{\textbf{Necessary}}
 In this part, we will prove that the two condition in theorem \ref{thm-assortment-hardness} is also necessary for revenue-order assortment to be optimal in every instance. Since the condition in \ref{thm-revenue-order-optimal} is necessary and sufficient, we will show that if none of the condition (a). $\mu \ge 1$ (b). $c 
 \ge 2\mu(1 -\mu)$ is satisfied, we can find an instance $I$ with product set $\{(r_i,p_i)\}_{i=1}^n$ such that the condition in theorem \ref{thm-revenue-order-optimal} cannot be satisfied.
 Intuitively, if $c$ is small relative to $\mu$,and $\mu$ is much smaller than $1$, then 
    function (\ref{equ-convex-function}) is strictly concave, so the inequality in lemma \ref{lem-convexity} will
    be converse. 
    
    Consider arbitrary convex weights $\alpha_j$ in  theorem \ref{thm-revenue-order-optimal} s.t. $\sum \alpha_j=1$ and satisfy 
    the two conditions so that theorem \ref{thm-revenue-order-optimal} will work, we will show that these $\alpha_j$ don't exist.
    
    The last equation in theorem \ref{thm-revenue-order-optimal} just says that
    \begin{equation}
        \begin{aligned}
            \sum_{k=1} ^n \alpha_k \lambda_k=\lambda_T
        \end{aligned}
    \end{equation}
    for incomplete set T.
   For any incomplete set T such that product $1$ is in $T$,
     set $j=1$ in theorem \ref{thm-revenue-order-optimal},  the following inequality  is satisfied
    \begin{equation} \label{equ-condition-for-1}
        \begin{aligned}
            \sum _{k=1}^n \alpha_k \frac {1}{\frac{\lambda_k}{1-\lambda_k}*\exp(\frac{c}{\mu-\lambda_k})+\exp(\frac{c}{\mu-\lambda_k})}\ge\frac {1}{\frac{\lambda_T}{1-\lambda_T}*\exp(\frac{c}{\mu-\lambda_T})+\exp(\frac{c}{\mu-\lambda_T})}
        \end{aligned}
    \end{equation}
    If 
$\mu<1$ and  $c<2 \mu (1-\mu)$, denote $F(x)$ as the second derivative of function \ref{equ-convex-function} such that $$F(x)=  c*\exp(-\frac{c}{\mu-x})*\frac {c(1-x)-2(1-\mu)(\mu-x)}{(\mu-x)^4}$$ then $F(0)<0$. So there exists $a<\mu$ such that in $[0,a]$, $F(x)<0$. Now we only need to design an instance $I$ with product set $\mathcal{N}=\{(r_i,p_i)\}_{i=1}^n$ such that $\lambda_{\mathcal{N}}<a$, then for instance $I$, the inequality \ref{equ-condition-for-1} will never be satisfied and we have a contradiction.
Given the equation \ref{equ-lambda},
it's obvious that we can easily design $\{(r_i,p_i)\}_{i=1}^n$ such that for any assortment $S$, we will have $\lambda_{S}<a$, and the proof is completed.
\QEDA

%%%%%%%%%%%%%%%%%%%%%%%%%%%%%%%%%%%%%%%%%%%%%%%%%%%%%%%%%%%%%%%%%%%%%%%%
\subsection{Proof of Theorem~\ref{thm-revenueorder-bound}}
\label{proof_thm:revenueorder-bound}
In this part, we will prove revenue-order assortment is $\frac{1}{3}$ optimal  for any instance $I$. Note that for assortment set $S$, the revenue can be written as 
$$R=\frac{\sum_{i \in S} p_i w_i}{\sum_{i \in S} w_i} \lambda$$
where $w_i=\exp(r_i-p_i)$ and  $\frac{\sum_{i \in S} p_i w_i}{\sum_{i \in S} w_i}$ can be regarded as average price.

Denote $S^{*}$ as the optimal assortment, and $p^{*}=\frac{\sum_{i \in S^{*}} p_i w_i}{\sum_{i \in S{*}} w_i}$ as the optimal average price. 
Then we first claim that: 

\noindent{\textbf{Observation}} All the product $i$ with price $p_i \ge p^*$ is in $S^{*}$. Otherwise adding these products will increase the revenue.

Without loss of generality, we assume that $p_1\ge \cdots \ge p_n$ and $p_k \ge p^* >p_{k+1}$. If $k\ge n-1$, we are already done. 
So in the following, we can divide $S^*= S_1 \bigcup S_2$, where 
$S_1=\{ i \in S^*, p_i \ge p^*\}$ (so $S_1$ is a revenue-order set) and $S_2=\{ i \in S^*, p_i < p^*\}$.
Similarly, we can define $\Bar{p}_1=\frac{\sum_{i \in S_1} p_i w_i}{\sum_{i \in S_1} w_i} $ and $\Bar{p}_2=\frac{\sum_{i \in S_2} p_i w_i}{\sum_{i \in S_2} w_i} $ as the average price of set $S_1$ and $S_2$. Besides, denote $\mathcal{W}_1=\sum_{i \in S_1} w_i$, $\mathcal{W}_2=\sum_{i \in S_2} w_i$ and $\mathcal{W}=\mathcal{W}_1+\mathcal{W}_2$, then the optimal revenue $R^*$ can be written as
\begin{equation}
    R^{*}=\frac{\Bar{p}_1 \mathcal{W}_1+ \Bar{p}_2 \mathcal{W}_2}{\mathcal{W}_1+\mathcal{W}_2} \lambda^{*}
\end{equation}
Besides, we will define $\lambda_1$ and $\lambda_2$ as the total purchasing rate decided by (\ref{equ-lambda}) when the assortment set is $S_1$ and $S_2$.  In the following, we will discuss different scenarios. 

\noindent{\textbf{Case 1: $\Bar{p}_1 \mathcal{W}_1 \ge c_1 p^{*}\mathcal{W}$}} 

In this case, we have $R(S_1) \ge c_1 R^{*}$. Considering \ref{equ-lambda}, we can observe that

\noindent{\textbf{Observation}} Regard $\lambda$ as a function of $\mathcal{W}$, $\frac{\lambda}{\mathcal{W}}$ is decreasing in $\mathcal{W}$.

So for assortment $S_1$,
\begin{equation}
    R(S_1)=\frac{\Bar{p}_1 \mathcal{W}_1}{\mathcal{W}_1} \lambda_1 \ge \frac{\Bar{p}_1 \mathcal{W}_1}{\mathcal{W}_1+\mathcal{W}_2} \lambda^{*} \ge c_1 R^{*}
\end{equation}
where the first inequality comes from the fact that $\frac{\lambda}{\mathcal{W}}$ is decreasing with $\mathcal{W}$, and the second comes from $\Bar{p}_1 \mathcal{W}_1 \ge c_1 p^{*}\mathcal{W}$.

\noindent{\textbf{Case 2: $\Bar{p}_1 \mathcal{W}_1 < c_1 p^{*}\mathcal{W}$} }

In this case, $\Bar{p}_2 \mathcal{W}_2 > (1-c_1)p^{*}\mathcal{W}$, so 
$\Bar{p}_2>(1-c_1) p^* \frac{\mathcal{W}}{\mathcal{W}_1}> (1-c_1) p^*$.
We can further divide $S_2$ into two subsets $S_3=\{i \in S_2, p_i \ge c_2 \bar{p}_2\}$, $S_4= \{i \in S_2, p_i <c_2 \Bar{p}_2\}$.
Similarly, we can define $\Bar{p}_3$, $\mathcal{W}_2$ and $\lambda_3$,  $\Bar{p}_4$, $\mathcal{W}_4$ and $\lambda_4$. Now consider the revenue-order assortment 
$S_{c_2 p_2}=\{i \in \mathcal{N}, p_i \ge c_2 p_2\}$.
We also consider two cases. Denote the set $S_{p^{*}, c_2 p_2}=\{ i \in \mathcal{N}, p^{*} > p_i \ge c_2 p_2\}$, so $S_{c_2 p_2}= S_1 \cup S_{p^*, c_2 p_2}$. For set $S_{p^{*}, c_2 p_2}$, we can also define 
$\Bar{p}_{p^*, c_2 p_2}$ as the average price in $S_{p^{*}, c_2 p_2}$
and $\mathcal{W}_{p^*, c_2 p_2}$ as the total utility.

\noindent{\textbf{Case 2.1} $\mathcal{W}_{p^*, c_2 p_2} \ge \mathcal{W}_2$ }

In this case,
\begin{equation}
    R(S_{c_2 p_2}) =\frac{p_1 \mathcal{W}_1 + \Bar{p}_{p^*, c_2 p_2}\mathcal{W}_{p^*, c_2 p_2} }{\mathcal{W}_{p^*, c_2 p_2}+\mathcal{W}_1} \lambda_{c_2 p_2} \ge c_2 p_2 \lambda^* \ge c_2(1-c_1) R^*
\end{equation}
where the first inequality comes from the following facts: 

\noindent(i) $\lambda_{c_2 p_2} \ge \lambda^{*}$ since $\mathcal{W}_{p^*, c_2 p_2}+\mathcal{W}_1> \mathcal{W}_{2}+\mathcal{W}_1=\mathcal{W}$.

\noindent (ii) $\frac{p_1 \mathcal{W}_1 + \Bar{p}_{p^*, c_2 p_2}\mathcal{W}_{p^*, c_2 p_2} }{\mathcal{W}_{p^*, c_2 p_2}+\mathcal{W}_1} \ge c_2 p_2$ since all the products have prices higher than $c_2 p_2$. 

The second inequality comes from $p_2 \ge (1-c_1) p^*$.

\noindent{\textbf{Case 2.2} $\mathcal{W}_{p^*, c_2 p_2} < \mathcal{W}_2$ }
\begin{equation}
    R(S_{c_2 p_2}) =\frac{p_1 \mathcal{W}_1 + \Bar{p}_{p^*, c_2 p_2}\mathcal{W}_{p^*, c_2 p_2} }{\mathcal{W}_{p^*, c_2 p_2}+\mathcal{W}_1} \lambda_{c_2 p_2} \ge (1-c_2) (1-c_1) R^{*}
\end{equation}
The bound comes from the following facts:

\noindent (i) $\frac{\lambda_{c_2 p_2}}{\mathcal{W}_{p^*, c_2 p_2}+\mathcal{W}_1} > \frac{\lambda^*}{\mathcal{W}}$ since $\mathcal{W}_{p^*, c_2 p_2}+\mathcal{W}_1< \mathcal{W}$ and $\frac{\lambda}{\mathcal{W}}$ is decreasing with $\mathcal{W}$.

\noindent (ii) $\Bar{p}_3 \mathcal{W}_3 +\Bar{p}_4 \mathcal{W}_4=\Bar{p}_2 \mathcal{W}_2$, so
\begin{equation}
    \Bar{p}_{p^*, c_2 p_2}\mathcal{W}_{p^*, c_2 p_2} =\sum_{i \in S_{p^*, c_2 p_2}} p_i w_i \ge \sum_{i \in S_3} p_i w_i \ge \Bar{p}_2 \mathcal{W}_2- c_2 \Bar{p}_2 \mathcal{W}_2= (1-c_2)\Bar{p}_2 \mathcal{W}_2 \ge (1-c_2) (1-c_1) p^* \mathcal{W}
\end{equation}
where the first inequality comes from $S_3 \subset S_{p^*, c_2p_2}$, the second inequality comes from the fact that the price of every product in $S_4$ is lower than $c_2 p_2$ and $\mathcal{W}_4 <\mathcal{W}_2$. The last inequality comes from $\Bar{p}_2 \mathcal{W}_2 \ge (1-c_1) p^* \mathcal{W}$.

Consider all three cases, we set $c_1=\frac{1}{3}$, $c_2=\frac{1}{2}$ and get a $\frac{1}{3}$ bound.
\QEDA

\subsection{Proof of Theorem~\ref{thm-homo-fptas}}
\label{proof_thm: homo-fptas}
In this part we will prove that the dynamic programming (\ref{equ-dp}) we propose is an \textit{FPTAS}. For any given pair $(f, g)$ with $f \leq f_{\max }, g \leq g_{\max }$, the dynamic program (\ref{equ-dp}) returns a feasible subset $S$ that satisfies the constraints (\ref{equ-constr}). Then, we have $\sum_{i \in S} \widetilde{w}_i \leq$ $k_{\max }:=\lfloor\bar{n} / \epsilon\rfloor+\bar{n}$, and then
$$
\sum_{i \in S} \frac{w_i}{\epsilon \underline{w}(1+\epsilon)^f / \bar{n}} \leq \sum_{i \in S}\left[\frac{w_i}{\epsilon \underline{w}(1+\epsilon)^f / \bar{n}}\right] \leq\lfloor\bar{n} / \epsilon\rfloor+\bar{n} .
$$
Immediately
$$
\sum_{i \in S} w_i \leq \frac{\lfloor\bar{n} / \epsilon\rfloor}{\bar{n} / \epsilon} \cdot \underline{w}(1+\epsilon)^f+\epsilon \underline{w}(1+\epsilon)^f \leq(1+\epsilon) \cdot \underline{w}(1+\epsilon)^f=\underline{w}(1+\epsilon)^{f+1}
$$
The last inequality holds because $\lfloor\bar{n} / \epsilon\rfloor /(\bar{n} / \epsilon) \leq 1$.  

For $\sum_{i \in S} \widetilde{p}_i \geq m_{\max }$, we consider
$$
\sum_{i \in S} \widetilde{p}_i=\sum_{i \in S}\left\lfloor\frac{p_i w_i}{\epsilon \underline{p}(1+\epsilon)^g / \bar{n}}\right\rfloor \geq m_{\max }:=\lfloor\bar{n} / \epsilon\rfloor-\bar{n} \Longrightarrow \sum_{i \in S} \frac{p_i w_i}{\epsilon \underline{p}(1+\epsilon)^g / \bar{n}} \geq\lfloor\bar{n} / \epsilon\rfloor-\bar{n} .
$$
Then, we have
$$
\sum_{i \in S}p_i w_i \geq \frac{\lfloor n / \epsilon\rfloor}{n / \epsilon} \cdot \underline{p}(1+\epsilon)^g-\epsilon \cdot \underline{p}(1+\epsilon)^g \geq(1-2 \epsilon) \underline{p}(1+\epsilon)^g .
$$
The last inequality holds because $\lfloor n / \epsilon\rfloor /(n / \epsilon) \geq 1-\epsilon$ for any $n \geq 1$.

On the other hand, if $\sum_{j \in S} w_i \leq \underline{w}(1+\epsilon)^f$ and $\sum_{i \in S}p_i w_i \geq \underline{p}(1+\epsilon)^g$, by scaling the inequality we have
$$
\begin{aligned}
    \sum_{i \in S} \frac{w_i}{\epsilon \underline{w}(1+\epsilon)^f / \bar{n}} \leq \frac{\bar{n}}{\epsilon} \Longrightarrow \sum_{i \in S}\left[\frac{w_i}{\epsilon \underline{w}(1+\epsilon)^f / \bar{n}}\right] \leq\left\lfloor\frac{\bar{n}}{\epsilon}\right\rfloor+\bar{n}:=k_{\max } \Longrightarrow \sum_{j \in S} \widetilde{w}_j \leq k_{\max }\\
\sum_{i \in S} \frac{p_i w_i}{\epsilon \underline{p}(1+\epsilon)^g / \bar{n}} \geq \frac{\bar{n}}{\epsilon} \Longrightarrow \sum_{i \in S}\left\lfloor\frac{p_iw_i}{\epsilon \underline{p}(1+\epsilon)^g / \bar{n}}\right\rfloor \geq\left\lfloor\frac{\bar{n}}{\epsilon}\right\rfloor-\bar{n}:=m_{\max } \Longrightarrow \sum_{j \in S} \widetilde{p}_j \geq m_{\max }
\end{aligned}
$$
Suppose that $S^*$ is an optimal solution to the assortment problem (\ref{equ-assortment}). There exist unique $f^*, g^*$ such that
$$
\begin{aligned}
& \underline{w}(1+\epsilon)^{f^*-1} \leq \sum_{i \in S^*} a_i<\underline{w}(1+\epsilon)^{f^*} \\
& \underline{p}(1+\epsilon)^{g^*-1} \leq \sum_{i \in S^*}p_i w_i<\underline{p}(1+\epsilon)^{g^*} .
\end{aligned}
$$
Then, for the combination of $\left(f^*-2, g^*\right)$, the dynamic program (\ref{equ-dp}) returns a feasible subset, denoted by $S^o$. By the above discussion, we have
$$
\begin{aligned}
& \sum_{i \in S^o} w_i \leq \underline{w}(1+\epsilon)^{f^*-2+1}=\underline{w}(1+\epsilon)^{f^*-1} \leq \sum_{i \in S^*} w_i \\
& \sum_{i \in S^o} p_i w_i \geq(1-2 \epsilon) \underline{p}(1+\epsilon)^{g^*} \geq(1-2 \epsilon) \cdot \sum_{i \in S^*} p_i w_i
\end{aligned}
$$
Denote $\lambda_{S^o}$ as the total purchasing rate with assortment $S^o$, $\mathcal{W}_{S^o}=\sum_{i \in S^o} w_i$.
The revenue for assortment $S^o$ is 
\begin{equation}
    R(S^o)=\frac{\sum_{i_in S^o} p_i w_i}{\mathcal{W}_{S^o}} \lambda_{S^o} \ge (1-2\epsilon) \frac{\sum_{i_in S^*} p_i w_i}{\mathcal{W}_{S^{*}}} \lambda_{S^*}=R^*
\end{equation} 
Since $\sum_{i_in S^o} p_i w_i \ge (1-2\epsilon) \sum_{i \in S^*} p_i w_i$ and $\frac{\lambda}{\mathcal{W}}$ is decreasing with $\mathcal{W}$
considering the equation (\ref{equ-lambda}).

For complexity of the dynamic programming, 
note that $f, g$ are bounded by $f_{\max }=O(\log (\bar{n} \bar{w} / \underline{w}) / \epsilon), g_{\max }=O(\log (\bar{n} \bar{p} / \underline{p}) / \epsilon)$, respectively; for any $(f, g)$, the size of the state space for each dynamic program (\ref{equ-dp-hetero}) is also bounded by $k_{\max }=\lfloor\bar{n} / \epsilon\rfloor+\bar{n}=O(\bar{n} / \epsilon)$ and $m_{\max }=\lfloor\bar{n} / \epsilon\rfloor-\bar{n}=O(\bar{n} / \epsilon)$. Therefore, its total running time is $O\left(\bar{n}^3 / \epsilon^5 \cdot \log (\bar{n} \bar{w} / \underline{w}) \cdot  \log (\bar{n} \bar{p} / \underline{p}) \right)$.
\QEDA

\subsection{Proof of Theorem~\ref{thm-hetero-fptas}}
\label{proof_thm: hetero-fptas}
 In this part, we will find \textit{FPTAS}  for the capacity constrained assortment optimization since assortment optimization (\ref{equ-assortment-hetero}) can be regarded as a special case with $K=|\mathcal{N}|=: \Bar{n}$. In order to simplify notation, we will use $w_i=\exp(r_i-p_i)$ for each service $i$.
    Let $\bar{w}=\max _{i \in \mathcal{N}} w_i,  \underline{w}=\min _{i \in \mathcal{N}} w_i ;  \bar{p}=\max _{i \in \mathcal{N}}p_i w_i,  \underline{p}=\min _{i \in \mathcal{N}}p_i w_i,  \bar{\alpha}=\max _{i \in \mathcal{N}}w_i/\mu_i,  \underline{\alpha}=\min _{i \in \mathcal{N}}w_i/\mu_i,  \bar{\beta}=\max _{i \in \mathcal{N}}w_i\mu_i^2,  \underline{\beta}=\min _{i \in \mathcal{N}}w_i/\mu_i^2$. For any positive $\epsilon$, define $f_{\max }=O(\log (n \bar{w} / \underline{w}) / \epsilon)$, $g_{\max }=O(\log (n \bar{p} / \underline{p}) / \epsilon)$, $h_{\max }=O(\log (n \bar{\alpha} / \underline{\alpha}) / \epsilon)$, $i_{\max }=O(\log (n \bar{\beta} / \underline{\beta}) / \epsilon)$. For any integer combination of $(f, g, h, i), f \leq f_{\max }$, $g \leq g_{\max }$, $h \leq h_{\max }$, $i \leq i_{\max }$ we discretize the coefficients as follows: for any $i \in \mathcal{N}$,
$$
\widetilde{w}_i=\left[\frac{w_i}{\epsilon \underline{w}(1+\epsilon)^f / n}\right\rceil,  \qquad \widetilde{p}_i=\left\lfloor\frac{p_i w_i}{\epsilon \underline{p}(1+\epsilon)^g / n}\right\rfloor ,\qquad \widetilde{\alpha}_i=\left\lfloor\frac{w_i/\mu_i}{\epsilon \underline{\alpha}(1+\epsilon)^h / n}\right\rfloor, \qquad \widetilde{\beta}_i=\left\lfloor\frac{w_i/ \mu_i^2}{\epsilon \underline{\beta}(1+\epsilon)^i / n}\right\rfloor
$$
where $\lfloor x\rfloor$ (resp., $\lceil x\rceil$ ) represents the largest (resp., smallest) integer that is not greater (resp., less) than $x$.
We want to find a subset $S \subseteq N$ such that
\begin{equation} \label{equ-constr-hetero}
    \sum_{i \in S} \widetilde{w}_i \leq j_{\max }  \qquad \sum_{i \in S} \widetilde{p}_i \geq m_{\max } \qquad \sum_{i \in S} \widetilde{\alpha}_i \leq k_{\max } \qquad \sum_{i \in S} \widetilde{\beta}_i \leq l_{\max }
\end{equation}

where $j_{\max }=k_{\max }=l_{\max }:\lfloor n / \epsilon\rfloor+n$ and $m_{\max }:=\lfloor n / \epsilon\rfloor-n$. For any possible combination of $(f,  g, h, l)$, we construct a subset $S$ as follows: for any integers $0 \leq j \leq j_{\max }, 0 \leq k \leq k_{\max },0 \leq l \leq l_{\max }, 0 \leq m \leq m_{\max }$ and $0 \leq n \leq \Bar{b}$,
\begin{equation}\label{equ-dp-hetero}
    H(j, k, l, m, n):=\min _{S \subseteq S_n}  |S|, \text { s.t., } \sum_{i \in S} \widetilde{w}_i \leq j,\quad \sum_{i \in S} \widetilde{\alpha}_i \leq k,\quad \sum_{i \in S} \widetilde{\beta}_i \leq l, \text { and } \sum_{i \in S} \widetilde{p}_i \geq m
\end{equation}
where $S_n:=\{1,2, \ldots, n\}$. 
At state $(j, k, l,  m, 0)$, let $H(j, k, l, m, 0)=0$ if $j, k, l \geq 0$ and $m \leq 0$, because the empty set is the only feasible solution for the constraints in the problem (\ref{equ-dp-hetero}); otherwise, a feasible solution for the constraints does not exist and let $H(j, k, l, m, 0)=\infty$. For any integers $0 \leq j \leq j_{\max }0 \leq k \leq k_{\max }, 0 \leq l \leq l_{\max }, 0 \leq m \leq m_{\max }$ and $1 \leq n \leq n$, we solve the problem (\ref{equ-dp-hetero}) by dynamic programming. The dynamic program is derived as follows:
$$
H(j, k,l,  m, n)=\min \left\{1+H\left(j-\widetilde{w}_n, k- \widetilde{\alpha}_n, l-\widetilde{\beta}_n, m-\widetilde{p}_n, n-1\right), H(j, k, l, m, n-1)\right\}
$$
If $H\left(j_{\max }, k_{\max }, l_{\max }, m_{\max }, n\right)\le K$, we find a feasible solution $S_{f,g, h, i}$ for constraints (\ref{equ-constr-hetero}). Then repeat the above procedure for all possible combinations of $(f,g,h,i)$. 
Therefore, we have $\sum_{i \in S} \widetilde{w}_i \leq$ $j_{\max }:=\lfloor\bar{n} / \epsilon\rfloor+\bar{n}$, and then
$$
\sum_{i \in S} \frac{w_i}{\epsilon \underline{w}(1+\epsilon)^f / \bar{n}} \leq \sum_{i \in S}\left[\frac{w_i}{\epsilon \underline{w}(1+\epsilon)^f / \bar{n}}\right] \leq\lfloor\bar{n} / \epsilon\rfloor+\bar{n} .
$$
Immediately
$$
\sum_{i \in S} w_i \leq \frac{\lfloor\bar{n} / \epsilon\rfloor}{\bar{n} / \epsilon} \cdot \underline{w}(1+\epsilon)^f+\epsilon \underline{w}(1+\epsilon)^f \leq(1+\epsilon) \cdot \underline{w}(1+\epsilon)^f=\underline{w}(1+\epsilon)^{f+1}
$$
The last inequality holds because $\lfloor\bar{n} / \epsilon\rfloor /(\bar{n} / \epsilon) \leq 1$. Similarly, we have
$$\sum_{i \in S} \alpha_i \leq \underline{\alpha}(1+\epsilon)^{h+1}, \qquad \sum_{i \in S} \beta_i \leq \underline{\beta}(1+\epsilon)^{i+1}$$
For $\sum_{i \in S} \widetilde{p}_i \geq m_{\max }$, we consider
$$
\sum_{i \in S} \widetilde{p}_i=\sum_{i \in S}\left\lfloor\frac{p_i w_i}{\epsilon \underline{p}(1+\epsilon)^g / \bar{n}}\right\rfloor \geq m_{\max }:=\lfloor\bar{n} / \epsilon\rfloor-\bar{n} \Longrightarrow \sum_{i \in S} \frac{p_i w_i}{\epsilon \underline{p}(1+\epsilon)^g / \bar{n}} \geq\lfloor\bar{n} / \epsilon\rfloor-\bar{n} .
$$
Then, we have
$$
\sum_{i \in S}p_i w_i \geq \frac{\lfloor n / \epsilon\rfloor}{n / \epsilon} \cdot \underline{p}(1+\epsilon)^g-\epsilon \cdot \underline{p}(1+\epsilon)^g \geq(1-2 \epsilon) \underline{p}(1+\epsilon)^g .
$$
The last inequality holds because $\lfloor n / \epsilon\rfloor /(n / \epsilon) \geq 1-\epsilon$ for any $n \geq 1$. 

On the other hand, if $\sum_{j \in S} w_i \leq \underline{w}(1+\epsilon)^f, \sum_{j \in S} w_i/\mu_i \leq \underline{\alpha}(1+\epsilon)^h, \sum_{j \in S} w_i/\mu_i^2 \leq \underline{\beta}(1+\epsilon)^i$ and $\sum_{i \in S}p_i w_i \geq \underline{p}(1+\epsilon)^g$, by scaling the inequality we have
$$
\begin{aligned}
    \sum_{i \in S} \frac{w_i}{\epsilon \underline{w}(1+\epsilon)^f / \bar{n}} \leq \frac{\bar{n}}{\epsilon} \Longrightarrow \sum_{i \in S}\left[\frac{w_i}{\epsilon \underline{w}(1+\epsilon)^f / \bar{n}}\right] \leq\left\lfloor\frac{\bar{n}}{\epsilon}\right\rfloor+\bar{n}:=j_{\max } \Longrightarrow \sum_{j \in S} \widetilde{w}_j \leq j_{\max }\\
\sum_{i \in S} \frac{p_i w_i}{\epsilon \underline{p}(1+\epsilon)^g / \bar{n}} \geq \frac{\bar{n}}{\epsilon} \Longrightarrow \sum_{i \in S}\left\lfloor\frac{p_iw_i}{\epsilon \underline{p}(1+\epsilon)^g / \bar{n}}\right\rfloor \geq\left\lfloor\frac{\bar{n}}{\epsilon}\right\rfloor-\bar{n}:=m_{\max } \Longrightarrow \sum_{j \in S} \widetilde{p}_j \geq m_{\max }\\
\sum_{i \in S} \frac{ w_i/\mu_i}{\epsilon \underline{\alpha}(1+\epsilon)^h / \bar{n}} \leq \frac{\bar{n}}{\epsilon} \Longrightarrow \sum_{i \in S}\left\lfloor\frac{w_i/\mu_i}{\epsilon \underline{\alpha}(1+\epsilon)^h / \bar{n}}\right\rfloor \leq\left\lfloor\frac{\bar{n}}{\epsilon}\right\rfloor+\bar{n}:=k_{\max } \Longrightarrow \sum_{j \in S} \widetilde{\alpha}_j \leq k_{\max }\\
\sum_{i \in S} \frac{ w_i/\mu_i^2}{\epsilon \underline{\beta}(1+\epsilon)^h / \bar{n}} \leq \frac{\bar{n}}{\epsilon} \Longrightarrow \sum_{i \in S}\left\lfloor\frac{w_i/\mu_i^2}{\epsilon \underline{\beta}(1+\epsilon)^h / \bar{n}}\right\rfloor \leq\left\lfloor\frac{\bar{n}}{\epsilon}\right\rfloor+\bar{n}:=l_{\max } \Longrightarrow \sum_{j \in S} \widetilde{\beta}_j \leq l_{\max }
\end{aligned}
$$
Suppose that $S^*$ is an optimal solution to the assortment problem (\ref{equ-assortment-hetero}). There exist unique $f^*, g^*, h^*, i^*$ such that
$$
\begin{aligned}
& \underline{w}(1+\epsilon)^{f^*-1} \leq \sum_{i \in S^*} a_i<\underline{w}(1+\epsilon)^{f^*} \\
& \underline{p}(1+\epsilon)^{g^*-1} \leq \sum_{i \in S^*}p_i w_i<\underline{p}(1+\epsilon)^{g^*} \\
& \underline{\alpha}(1+\epsilon)^{h^*-1} \leq \sum_{i \in S^*}w_i/\mu_i<\underline{\alpha}(1+\epsilon)^{h^*} \\
& \underline{\beta}(1+\epsilon)^{i^*-1} \leq \sum_{i \in S^*}w_i/\mu_i^2<\underline{\beta}(1+\epsilon)^{i^*} 
\end{aligned}
$$
Then, for the combination of $\left(f^*-2, g^*, h^*-2, i^*-2\right)$, the dynamic program (\ref{equ-dp}) returns a feasible subset, denoted by $S^o$. By the above discussion, we have
$$
\begin{aligned}
& \sum_{i \in S^o} w_i \leq \underline{w}(1+\epsilon)^{f^*-2+1}=\underline{w}(1+\epsilon)^{f^*-1} \leq \sum_{i \in S^*} w_i \\
& \sum_{i \in S^o} p_i w_i \geq(1-2 \epsilon) \underline{p}(1+\epsilon)^{g^*} \geq(1-2 \epsilon) \cdot \sum_{i \in S^*} p_i w_i\\
& \sum_{i \in S^o} w_i/\mu_i \leq \underline{\alpha}(1+\epsilon)^{h^*-2+1}=\underline{\alpha}(1+\epsilon)^{h^*-1} \leq \sum_{i \in S^*} w_i/\mu_i\\
& \sum_{i \in S^o} w_i/\mu_i^2 \leq \underline{\beta}(1+\epsilon)^{i^*-2+1}=\underline{\beta}(1+\epsilon)^{i^*-1} \leq \sum_{i \in S^*} w_i/\mu_i^2
\end{aligned}
$$
Denote the total revenue given assortment $S$ as $R(S)$, the total purchasing rate with optimal assortment $S^*$ as $\lambda^*$ and the total with assortment $S^o$ as $\lambda^o$. Besides, denote $\mathcal{W}^*= \sum_{i \in S^*} w_i$ and  $\mathcal{W}^o= \sum_{i \in S^o} w_i$.  
we claim that 
\begin{lemma}\label{lem-hetero-lambda}
    \begin{equation}
        \frac{\lambda^*}{\mathcal{W}^*} \le \frac{\lambda^o}{\mathcal{W}^o}
    \end{equation}
\end{lemma}
\noindent{\textbf{Proof}} 
Consider the choice model (\ref{equ-heterowait}), we can rewrite it as 
\begin{equation}\label{equ-lambda-hetero}
    \frac{\mathcal{W}}{\lambda}= \mathcal{W}+ \exp(c\frac{\sum_{i \in S} \frac{w_i}{\mu_i^2} \frac{\lambda}{\mathcal{W}}}{1-\sum_{i \in S} \frac{w_i}{\mu_i} \frac{\lambda}{\mathcal{W}}})
\end{equation}
where $\mathcal{W}=\sum_{i \in S} w_i$ and $\lambda=\sum_{i \in S} \lambda_i$ is the total purchasing rate. Using (\ref{equ-lambda-hetero}), and note that $\sum_{i \in S^o} w_i\le \sum_{i \in S^*} w_i $, $\sum_{i \in S^o} w_i/\mu_i\le \sum_{i \in S^*} w_i/\mu_i$, $\sum_{i \in S^o} w_i/\mu_i^2\le \sum_{i \in S^*} w_i/\mu_i^2$, we can see that
$ \frac{\lambda^*}{\mathcal{W}^*} \le \frac{\lambda^o}{\mathcal{W}^o}$.
\qed

With lemma \ref{lem-hetero-lambda}, and note that $\sum_{i \in S^o} p_i w_i \ge (1-2\epsilon) \sum_{i \in S^*} p_i w_i$, denote $R(S)$ as the revenue given assortment set $S$, we have
\begin{equation}
    R(S^o)=\sum_{i \in S^o} p_i w_i \frac{\lambda^o}{\mathcal{W}^o} \ge
   (1-2\epsilon) \sum_{i \in S^*} p_i w_i \frac{\lambda^*}{\mathcal{W}^*}=(1-2\epsilon)R(S^*)
\end{equation}
For complexity of the dynamic programming, 
note that $f, g, h$ and $i$ are bounded by $f_{\max }=O(\log (\bar{n} \bar{w} / \underline{w}) / \epsilon), g_{\max }=O(\log (\bar{n} \bar{p} / \underline{p}) / \epsilon), h_{\max }=$ $O(\log (\bar{n} \bar{\alpha} / \underline{\alpha}) / \epsilon)$ and $ i_{\max }=$ $O(\log (\bar{n} \bar{\beta} / \underline{\beta}) / \epsilon)$, respectively; for any $(f, g, h, i)$, the size of the state space for each dynamic program (\ref{equ-dp-hetero}) is also bounded by $j_{\max }=k_{\max }=l_{\max }=\lfloor\bar{n} / \epsilon\rfloor+\bar{n}=O(\bar{n} / \epsilon)$ and $m_{\max }=\lfloor\bar{n} / \epsilon\rfloor-\bar{n}=O(\bar{n} / \epsilon)$. Therefore, its total running time is $O\left(\bar{n}^5 / \epsilon^7 \cdot \log (\bar{n} \bar{w} / \underline{w})  \cdot \log (\bar{n} \bar{p} / \underline{p})  \cdot \log (\bar{n} \bar{\alpha} / \underline{\alpha}) \cdot \log (\bar{n} \bar{\beta} / \underline{\beta}) \right)$.

\QEDA

\subsection{Proof of Lemma~\ref{lem-consumer-surplus}}
\label{proof: lem-consumer-surplus}
 For classic MNL model, consumer surplus will be
 $$\log (1+\sum_{i=1}^n\exp(r_i-p_i))$$
 which is log-sum of the anticipated utility for every choice (including outside option with utility 1). 
 In our setting, the anticipated utility is decided by 
 $$
u_{i}=r_{i}-p_{i}-c\left(\Tilde{\mathbb{E}}[W_i]\right)+ \xi_i
$$
where for non-priority queue, $\Tilde{\mathbf{E}}[W_i]=\mathbb{E}[W_i] +\frac{1}{\mu_i}=\frac{\sum_{k=1}^n \lambda_{k} / \mu_{k}^{2}}{1-\sum_{k=1}^n \lambda_{k} / \mu_{k}}+\frac{1}{\mu_{i}}$ and for priority queue, $ \Tilde{\mathbb{E}}[W_{i_k}]=\frac{\sum_{j=1}^k \lambda_{i_j} / \mu_{i_j}^{2}}{(1-\sum_{j=1}^k \lambda_{i_j} / \mu_{i_j})(1-\sum_{j=1}^{k-1} \lambda_{i_j} / \mu_{i_j})}+\frac{1}{\mu_{i_k}(1-\sum_{j=1}^{k-1} \lambda_{i_j} / \mu_{i_j})}$ for the product with $k^{th}$ priority.
So for both priority and non-priority queue, the total purchasing rate $\lambda$ is decided by
\begin{equation}
    \lambda=\frac{\sum_{k=1}^n \exp \left(r_{k}-p_{k}-c_{k} \tilde{\mathbb{E}}(W_{k})\right)}{1+\sum_{k=1}^n \exp \left(r_{k}-p_{k}-c_{k} \tilde{\mathbb{E}}(W_{k})\right)}
\end{equation}
while $\tilde{\mathbb{E}}$ is different in priority queue and same in non-priority queue.
 So for both settings, the consumer surplus can be formulated as
 $$\log(1 +\sum_{i=1}^n\exp(r_i-p_i-c\Tilde{\mathbb{E}}(W_i)))=-\log(1-\lambda)$$
 \QEDA

\subsection{Proof of Theorem~\ref{thm-cmu}}
\label{proof_thm: cmu}
Note that the joint pricing and priority assortment optimization can characterized as
\begin{equation}
   \max_{\boldsymbol{\lambda},(i_1, \cdots, i_n) }\pi(\boldsymbol{\lambda},\lambda)=\sum_{j=1}^n \lambda_{i_j}(r_{i_j}-\log(\lambda_{i_j}))+\lambda \log(1-\lambda)- \sum_{j=1}^n
   c_{i_j}  \lambda_{i_j}\mathbb{E}(W_{i_j})
\end{equation}
For given $(\lambda_{i_j})_{j=1}^n$, we optimize over all possible priority assignment $(i_1, \cdots, i_n)$. Since the priority assignment only impacts the expected waiting time $\mathbb{E}(W_{i_j})$, and $\sum_{j=1}^n
   c_{i_j}  \lambda_{i_j}\mathbb{E}(W_{i_j})$ is exactly the total waiting cost. So for any given  $(\lambda_{i_j})_{j=1}^n$, serving
   the order with largest $c_j \mu_j$ minimizes waiting cost, and therefore maximizes revenue by classic $c\mu$-rule. The waiting cost is also lower than non-priority queue as stated in $c\mu$-rule.  Then with fixed priority assignment, we optimize over $\lambda_{i_1}, \cdots, \lambda_{i_n}$ and find the optimal purchasing rate and the optimal price.
\QEDA

\subsection{Proof of Corollary~\ref{cor-priority-special-case}}
\label{proof_cor: priority-special-case}
In the special case where $c_i=c$ and $\mu_i=\mu$, we can characterize the expected waiting time for product with $j^{th}$ priority as:
$$\mathbb{E}(W_{i_j})=\frac{c}{\mu-\sum_{j=1}^{i-1}\lambda_{j}} \cdot \frac{\mu}{\mu-\sum_{j=1}^{i}\lambda_{j}}$$
Therefore, the joint pricing and assortment optimization can be characterized as:
\begin{equation}\label{equ-priority-special-case}
\begin{aligned}
    \max_{\boldsymbol{\lambda},(i_1,\cdots,i_n)} \pi(\boldsymbol{\lambda},\lambda)&=\sum_{j=1}^n \lambda_{i_j}(r_{i_j}-\lambda_{i_j})+\lambda \log(1-\lambda)- \sum_{j=1}^n
   c_{i_j}  \lambda_{i_j}\mathbb{E}(W_{i_j})\\
   &=\sum_{j=1}^{n} \lambda_{i_j}\left(r_{i_j}-\log \lambda_{i_j}\right)+\log \left(1-\lambda\right) \lambda-c\left(\frac{\lambda}{\mu(\mu-\lambda)}+\frac{\lambda}{\mu}\right)\\
   \text{sub to.  } &\sum_{j=1}^n \lambda_{i_j} < \min\{1,\mu\}
\end{aligned}
\end{equation}
Note that in (\ref{equ-priority-special-case}), given $(\lambda_{1}, \cdots. \lambda_n)$ the total waiting cost is the same as non-priority case no matter how priority is assigned. Therefore, the priority assignment doesn't matter and the optimal $\lambda_i$ is exactly the same as proposition \ref{prop-optpric}  in non-priority case. But with priority the optimal price for product with $j^{th}$ priority is given by
\begin{equation}
     p_{i_j}=\log \sum_{j=1}^{n} e^{r_{j}}-\log \lambda^{*}+\log \left(1-\lambda^{*}\right)-\frac{c}{\mu-\sum_{k=1}^{j-1}\lambda_{i_k}^*} \cdot \frac{\mu}{\mu-\sum_{k=1}^{j}\lambda_{i_k}^*}
 \end{equation}
 We can find that the only difference in optimal price comes from the expected waiting cost. With higher priority, the service needs to be paid more for shorter waiting time.
\QEDA

\subsection{Proof of Proposition~\ref{prop-rev-compare}}
\label{proof_prop: rev-compare}
In this part, we will compare the revenue under disclosure and non-disclosure setting. 
Note that for any $L$, $i$, $j$,
$\frac {\lambda_{L,i}}{\lambda_{L,j}}=\frac{exp(r_i-p_i)}{exp(r_j-p_j)}$. This is similar to nondisclosure setting. So we will first focus on the total purchasing rate $\Lambda_L$, and
denote $\sum_{i=1}^{n}exp(r_i-p_i)=\mathcal{W}$, we get that:
\begin{equation}
\lambda_{L}=\frac{\mathcal{W}}{\exp \left(c \cdot \frac{L+1}{\mu}\right)+\mathcal{W}}
\end{equation}
Together with (\ref{equ-birth-and-death}), the expected purchasing rate will be:
\begin{equation} \label{equ-lambda-dis}
\begin{aligned}
\hat{\lambda}=\sum_{i=0}^{\infty} P_i \cdot \lambda_i= \mu \cdot (1-P_0)
\end{aligned}
\end{equation}
Now notice that the nondisclosure purchasing rate will satisfy the function:
\begin{equation}
\mathcal{W}=\exp \left(\frac{c}{\mu-\lambda}\right) \frac{\lambda}{1-\lambda}
\end{equation}
So, disclosure will benefit if and only if the following inequality is satisfied:
    \begin{equation}
\mathcal{W}<\exp \left(\frac{c}{\mu-\hat{\lambda}}\right) \frac{\hat{\lambda}}{1-\hat{\lambda}}
\end{equation}
where $\hat{\lambda}$ is defined from equation (\ref{equ-lambda-dis}).

In the following, we will show that when $\mu$ is small, disclosure will benefit, while when $\mu$ is large nondisclosure will make more revenue.

\noindent{\textbf{Part I}}    Given  $c, \mathcal{W}$, when $\mu$ is smaller than a threshold $l(c, \mathcal{W})$, disclosure will make more revenue 

\noindent{\textbf{Proof}} In proposition \ref{prop-aymp-monotone}, we prove that for given $\mathcal{W}$, there exists a threshold $h(\mathcal{W})$ such that
when $c/\mu >h(\mathcal{W})$, the revenue is increasing with the threshold $L$ for disclosure strategy and this part of proposition \ref{prop-rev-compare} is contained since 
$F(0) < F(\infty)$. So we can just set $l(c,\mathcal{W})=c/h(\mathcal{W})$ and get our result.

\noindent{\textbf{Part II}}
    Given c and W, when $\mu$ is bigger than a threshold , nondisclosure will make more revenue 

\noindent{\textbf{Proof}}   Note that

    \begin{equation}
        \begin{aligned}
        \exp \left(\frac{c}{\mu-\hat{\lambda}}\right) =\exp(\frac{c}{\mu} (1+\sum_{i=1}^{\infty} \prod_{j=0}^{i-1}\frac{\lambda_j}{\mu})) \le \exp(\frac{c}{\mu} (1+\sum_{i=1}^{\infty}(\frac{\lambda_0}{\mu})^i))  \le
        \exp(\frac{c}{\mu-\lambda_0} )
        \end{aligned}
    \end{equation}
    Here we assumed $\mu>1$ to guarantee convergence.
    And also note that
     \begin{equation}
        \begin{aligned}
       \frac{\hat{\lambda}}{1-\hat{\lambda}}=\frac{\mu(1-P_0)}{1-\mu(1-P_0)}=\frac{\mu(\sum_{i=1}^{\infty} \prod_{j=0}^{i-1}\frac{\lambda_j}{\mu})}{\mu+(1-\mu)(\sum_{i=1}^{\infty} \prod_{j=0}^{i-1}\frac{\lambda_j}{\mu})} \le 
       \frac{\sum_{i=1}^{\infty} \prod_{j=0}^{i-1}\frac{\lambda_j}{\mu}}{1-(\sum_{i=1}^{\infty} \prod_{j=0}^{i-1}\frac{\lambda_j}{\mu})}\le \frac{\frac{W}{\mu(W+\exp(\frac{c}{\mu}))}}{1-2\frac{W}{\mu(W+\exp(\frac{c}{\mu}))}}
        \end{aligned}
    \end{equation}
   So  when $\mu$ is bigger than a threshold $r(c,\mathcal{W})$, 
   $\exp(\frac{c}{\mu-\lambda_0} )\frac{\frac{W}{\mu(W+\exp(\frac{c}{\mu}))}}{1-2\frac{W}{\mu(W+\exp(\frac{c}{\mu}))}} < \mathcal{W}$, and  non-disclosure will have higher revenue.  
\QEDA

\subsection{Proof of Lemma~\ref{lem-P0-dis}}
\label{proof_lem: P_0-dis}
For the general class of disclosure policy with threshold $L$, the state of queue length can still be regarded as a birth-and-death process, with transition rate $\lambda_L$ from $l$ to $l+1$ for all $0 \le l< L$, $\lambda_L^{'}$ from $l $ to $l+1$  for all $l \ge L$ and $\mu$ from $l+1$ to $ l$ for every $l \ge 0$. Therefore, the birth and death process can be characterized as
\begin{equation}\label{equ-P0-def}
\begin{aligned}
        P_0&=\frac{1}{1+\frac{\lambda_0}{\mu}+\cdots +
\frac{\prod_{i=1}^{L-1}\lambda_i}{\mu^L}\cdot\frac{ \lambda_L^{\prime}}{(\mu-\lambda_L^{\prime})}}\\
  P_j& = \frac{\lambda_{j-1}}{\mu} P_{j-1} \text{ for    }  j \le L\\
  P_j& = \frac{\lambda_{L}^{\prime}}{\mu} P_{j-1} \text{ for    }  j > L
\end{aligned}
\end{equation}
And the total purchasing rate 
\begin{equation}\label{equ-hatlambda}
    \hat{\lambda}=\sum_{i=0}^{\infty} P_i \cdot \lambda_i= \mu \cdot (1-P_0)
\end{equation}
\QEDA

\subsection{Proof of Proposition~\ref{prop-aymp-monotone}}
\label{proof_prop: aymp-monotone}
We first prove that the total purchasing rate is asymptotically increasing, and $F(\infty)$ is a local maximum. Then we will prove that given $\mathcal{W}$, when $c/\mu$ is large enough, total purchasing rate is increasing with threshold $k$, and $F(\infty)$ is globally optimal. Denote $t_k=\frac{(K+1)c}{\mu}+\frac{c\lambda^{'}_k}{\mu(\mu-\lambda^{'}_k)}$, then we  know that
$$\lambda_k^{'}=\frac{\mathcal{W}}{\exp(t_k)+\mathcal{W}}$$
We have the following claims:

\noindent{\textbf{Claim 1}} $\lambda_k^{\prime}$ and $\lambda_k$ are decreasing with $k$ and converges to $0$.

\noindent{\textbf{Claim 2}} Given that $\lambda_k^{\prime}$ is 
characterized as 
$$
\mathcal{W}=\exp \left(c\frac{k+1}{\mu}+\frac{c\lambda_k^{\prime}}{\mu(\mu-\hat{\lambda})}\right) \frac{\lambda_k^{\prime}}{1-\lambda_k^{\prime}}
$$
So given fixed $\mathcal{W}, k\ge0$, $\exp \left(c\frac{k+1}{\mu}+\frac{c\lambda_k^{\prime}}{\mu(\mu-\hat{\lambda})}\right) \ge O(\exp(\frac{c}{\mu}))$ as $\frac{c}{\mu} \rightarrow \infty$ so $\frac{\lambda_k^{\prime}}{1-\lambda_k^{\prime}}\le \boldsymbol{O}(\exp(-\frac{c}{\mu}))$ and thus $\lambda_k^{\prime}\le \boldsymbol{O}(\exp(-\frac{c}{\mu}))$.

Therefore, we can characterize $\frac{\lambda_k}{\mu-\lambda_{k+1}^{\prime}}-\frac{\lambda_{k}^{\prime}}{\mu-\lambda_{k}^{\prime}}$ as
\begin{equation}\label{equ-monotone-equiv}
\begin{aligned}
    \frac{\lambda_k}{\mu-\lambda_{k+1}^{\prime}}-\frac{\lambda_{k}^{\prime}}{\mu-\lambda_{k}^{\prime}}>0  &\Longleftrightarrow \frac{\mathcal{W}}{(\exp(\frac{(k+1)c}{\mu})+\mathcal{W})(\mu-\lambda_{k+1}^{\prime})}-\frac{\mathcal{W}}{(\exp(t_k)+\mathcal{W})(\mu-\lambda_{k}^{\prime})}>0\\
    &\Longleftrightarrow \frac{\exp(t_k)+\mathcal{W}}{\mu-\lambda_{k+1}^{\prime}} -\frac{\exp(\frac{(k+1)c}{\mu}+\mathcal{W}}{\mu-\lambda_{k}^{\prime}}>0\\
    &\Longleftrightarrow` \frac{\exp(t_k)-\exp(\frac{(k+1)c}{\mu})}{\mu-\lambda_{k+1}^{\prime}}+ \frac{(\mathcal{W}+\exp(\frac{(k+1)c}{\mu}))(\lambda_{k+1}^{\prime}-\lambda_k^{\prime})}{(\mu-\lambda_{k}^{\prime})(\mu-\lambda_{k+1}^{\prime})}>0
\end{aligned}
\end{equation}

The first part of the last inequality in  \ref{equ-monotone-equiv} can be formulated as
\begin{equation*}
    \frac{\exp(t_k)-\exp(\frac{(k+1)c}{\mu})}{\mu-\lambda_{k+1}^{\prime}} \ge \frac{\exp(\frac{(k+1)c}{\mu})\frac{c\lambda^{'}_k}{\mu(\mu-\lambda^{'}_k)}}{\mu-\lambda_{k+1}^{\prime}}=\frac{\exp(\frac{(k+1)c}{\mu})}{(\mu-\lambda_{k+1}^{\prime})(\mu-\lambda_{k+1}^{\prime})} \frac{c \lambda_n^{\prime}}{\mu}
\end{equation*}
where the first inequality holds since $e^x-1\ge x$.
For the second part, note that 
\begin{equation}\label{equ-asymp-lambda}
    \frac{\mathcal{W}+\exp(\frac{(k+1)c}{\mu}}{\exp(\frac{(k+1)c}{\mu}}=\frac{1}{1-\lambda_k^{\prime}}
    =1+\boldsymbol{O}(\lambda_k^{\prime}) 
\end{equation}
when $\lambda_k^{\prime}$ is small enough, so the second part 
can be formulated as 
\begin{equation}
    \frac{(\mathcal{W}+\exp(\frac{(k+1)c}{\mu}))(\lambda_{k+1}^{\prime}-\lambda_k^{\prime})}{(\mu-\lambda_{k}^{\prime})(\mu-\lambda_{k+1}^{\prime})}= \frac{\exp(\frac{(k+1)c}{\mu})(1+\boldsymbol{O}(\lambda_k^{\prime}))(\lambda_{k+1}^{\prime}-\lambda_k^{\prime})}{(\mu-\lambda_{k}^{\prime})(\mu-\lambda_{k+1}^{\prime})}
\end{equation}
so combining two parts together, the last inequality in \ref{equ-monotone-equiv} can be characterized as
\begin{equation}
\begin{aligned}\label{equ-monotone-equiv2}
     \frac{\exp(t_k)-\exp(\frac{(k+1)c}{\mu})}{\mu-\lambda_{k+1}^{\prime}}+ \frac{(\mathcal{W}+\exp(\frac{(k+1)c}{\mu}))(\lambda_{k+1}^{\prime}-\lambda_k^{\prime})}{(\mu-\lambda_{k}^{\prime})(\mu-\lambda_{k+1}^{\prime})} &\ge \frac{\exp(\frac{(k+1)c}{\mu})}{(\mu-\lambda_{k+1}^{\prime})(\mu-\lambda_{k+1}^{\prime})} \frac{c \lambda_n^{\prime}}{\mu} +\frac{\exp(\frac{(k+1)c}{\mu})(1+\boldsymbol{O}(\lambda_k^{\prime}))(\lambda_{k+1}^{\prime}-\lambda_k^{\prime})}{(\mu-\lambda_{k}^{\prime})(\mu-\lambda_{k+1}^{\prime})}\\
    & = \frac{\exp(\frac{(k+1)c}{\mu}) (\lambda_{k+1}^{\prime}-(1-\frac{c}{\mu})\lambda_{k}^{\prime}+ \boldsymbol{O}(\lambda_k^{\prime})^2)}{(\mu-\lambda_{k}^{\prime})(\mu-\lambda_{k+1}^{\prime})}
     \end{aligned}
\end{equation}
%%%%%%%%%%%%%%%%%%%%%%%%%%%%%%%%%%
%%%%%%%%%%%%%%%%%%%%%%%%%%%%%%%%%%
%%%%%%%%%%%%%%%%%%%%%%%%%%%%%%%%%%
%
Now note that
\begin{equation}\label{equ-aymp-ratio}
    \exp \left(c\frac{k+2}{\mu}+\frac{c\lambda_{k+1}^{\prime}}{\mu(\mu-\lambda_k^{\prime})}\right) \frac{\lambda_{k+1}^{\prime}}{1-\lambda_{k+1}^{\prime}}=\mathcal{W}=\exp \left(c\frac{k+1}{\mu}+\frac{c\lambda_k^{\prime}}{\mu(\mu-\hat{\lambda})}\right) \frac{\lambda_k^{\prime}}{1-\lambda_k^{\prime}}
\end{equation}
and in claim 1 we prove that $\lambda_k^{\prime} \rightarrow 0$, so we compare the two side in equation \ref{equ-aymp-ratio} and can find that $\lim_{k \rightarrow \infty} \lambda_{k+1}^{\prime}/\lambda_{k}^{\prime}=\exp(-c/\mu)$.
Finally consider the last equation of \ref{equ-monotone-equiv2}, since $\exp(-c/\mu)>1-c/\mu$ as $e^x>1+x$ for any $x<0$ and $\boldsymbol{O}(\lambda_k^{\prime})^2=\boldsymbol{o}(\lambda_k^{\prime})$ as 
$k\rightarrow \infty$, we prove that $\lambda_{k+1}^{\prime}-(1-\frac{c}{\mu})\lambda_{k}^{\prime}+ \boldsymbol{O}(\lambda_k^{\prime})^2\ge 0$ and $F(k+1)-F(k)\ge0$ for large enough $k$. Therefore, the total market share for disclosure policy is aymptotically increasing. 

Now we prove the second part of proposition \ref{prop-aymp-monotone}, that is $F(k+1)-F(k)\ge 0$ for any $k\ge 0$. Just go through the proof above, we can see that for any given $k$, 
if we want to prove  $F(k+1)-F(k)\ge 0$, we only need to make sure that  \ref{equ-asymp-lambda} holds, and that
$\lambda_{k+1}^{\prime}-(1-\frac{c}{\mu})\lambda_{k}^{\prime}+ \boldsymbol{O}(\lambda_k^{\prime})^2\ge 0$ in \ref{equ-monotone-equiv2} holds. For the first part, note that $\lambda_k^{\prime}\le \exp(-c/\mu) $, so when $c/\mu$ is large enough, $\lambda_k^{\prime}$ is small enough such that $\frac{1}{1-\lambda_k^{\prime}}<1+2\lambda_k^{\prime}$ so \ref{equ-asymp-lambda} holds.
For the second part, we can also see that when $c/\mu$ is large enough, $(\frac{c}{\mu}-1)\lambda_{k}^{\prime}-2 (\lambda_k^{\prime})^2>0$ holds, thus $F(k+1)-F(k)\ge0$ for any $k$, and the total market share is increasing with disclosure threshold $k$, thus full-disclosure is optimal.
\QEDA

\subsection{Proof of Proposition~\ref{prop-pricing-dis}}
\label{proof_prop: pricing-dis}
In this part, we will find the optimal pricing strategy under disclosure setting. First of all, we will prove that the optimal price for each product is equal. Similar to non-disclosure case, we first formulate price for product $p_i$ in terms of purchasing rate $\lambda_i$ and total purchasing rate $\lambda$. In particular, when the queue length is $L$, $p_i$ can be formulated as 
\begin{equation}\label{equ-price-dis}
    p_{i}(\boldsymbol{\lambda})=r_{i}-\log \lambda_{i,L}+\log \left(1-\sum_{j=1}^{n} \lambda_{j,L}\right)-\frac{c(L+1)}{\mu}
\end{equation}
Therefore, for any $L$, $L+1$, 
\begin{equation}\label{equ-price-dis-equiv}
   r_{i}-\log \lambda_{i,L}+\log \left(1-\sum_{j=1}^{n} \lambda_{j,L}\right)-\frac{c(L+1)}{\mu}= p_{i}(\boldsymbol{\lambda})=r_{i}-\log \lambda_{i,L+1}+\log \left(1-\sum_{j=1}^{n} \lambda_{j,L+1}\right)-\frac{c(L+2)}{\mu}
\end{equation}
or equivalently, 
\begin{equation}\label{equ-dis-lambdaratio}
    \frac{\lambda_{i,L}}{1-\lambda_L}=\exp(\frac{c}{\mu})  \frac{\lambda_{i,L+1}}{1-\lambda_{L+1}}
\end{equation}
Sum over $i$, we have 
\begin{equation}\label{equ-dis-lambdaratio2}
    \frac{\lambda_{L}}{1-\lambda_L}=\exp(\frac{c}{\mu})  \frac{\lambda_{L+1}}{1-\lambda_{L+1}}
\end{equation}
Therefore, once $\lambda_0$ is determined, $\lambda_L$ is fixed, and therefore $P_L$ is fixed where $P_L$ is the probability for the queue length to be $L$ for any $L\ge 0$. Compare \ref{equ-dis-lambdaratio} and \ref{equ-dis-lambdaratio2}, we can also see that $\lambda_{i,L}/\lambda_{L}=\lambda_{i,L+1}/\lambda_{L+1}$ for any $L\ge 0$.
Now the pricing optimization problem can be written as
\begin{equation}
\begin{aligned}\label{equ-lambda-optimization}
    \max_{\lambda_L,\boldsymbol{\lambda}_L=\{\lambda_{L,i}\}_{i=1}^n} &\sum_{L=0}^{\infty} P_L 
    \left(\sum_{i=1^n}\lambda_{i,L}(r_i-\log(\lambda_{i,L})+ \lambda_L \log(1-\lambda_L)-\lambda_L \cdot c\frac{L+1}{\mu}\right)\\
    \text{sub. to.   } &\sum_{i=1}^n \lambda_{L,i}=\lambda_L \text{  for any }L\\
    & \frac{\lambda_{L,i}}{\lambda_L}=\frac{\lambda_{0,i}}{\lambda_0} \text{  for any }L
\end{aligned}
\end{equation}
Note that here $P_L$ is determined by only $\lambda_0$ but not 
$\lambda_{0,i}$. So now note that for any fixed $\lambda_0$, $\lambda_L$ and $P_L$ are fixed. Consider the optimization of 
$\sum_{i=1^n}\lambda_{i,L}(r_i-\log(\lambda_{i,L})$ with constraint $\sum_{i=1}^n \lambda_{L,i}=\lambda_L$ for any $L$, the optimal $\lambda_{i,L}$ satisfies 
\begin{equation}
    \lambda_{i,L}=\frac{e^{r_i}}{\sum_{i=1}^n e^{r_i}}\lambda_L
\end{equation}
for any $i$ and $L$. Note that this solution also satisfies the constraint $\frac{\lambda_{L,i}}{\lambda_L}=\frac{\lambda_{0,i}}{\lambda_0} $ in \ref{equ-lambda-optimization}, so we know that the optimal solution $\lambda_{i,L}$ satisfies that 
$r_i-\lambda_{i,L}=r_j-\lambda_{j,L}$ for any $i,j ,L$, and therefore the optimal price $p_i=p_j$ for any $i,j$.
So now denote the optimal price as $p^{*}$, and given that
the total revenue can be written as
$$R=p \hat{\lambda}$$ where $\hat{\lambda}$ is the total purchasing rate which is given in \ref{equ-hatlambda} and \ref{equ-P0-def}.
Note that in this case $\lambda_L$ can be written as $$\frac{W^{'}}{\exp(\frac{c (j+1)}{\mu}+p)+W^{'}}$$,
where $W^{'}=\sum_{i=1}^n \exp(r_i)$, the pricing optimization problem can be defined as
\begin{equation}
     \max_{p \ge 0} R(p)=p \cdot (1-\frac{1}{1+\sum_{i=1}^{\infty}
           \prod_{j=0}^{i} \frac{W^{'}}{\exp(\frac{c (j+1)}{\mu}+p)+W^{'}} \cdot \frac{1}{\mu^i}})
\end{equation}
Now we prove that $R(p)$ is a concave function of $p$, which tells us that $R(p)$ is also uni-modal since $R(p)=0$ and $R(\infty)=0$.
\begin{equation}
    R^{\prime}(p)=1-\frac{1}{1+\sum_{i=1}^{\infty}
           \prod_{j=0}^{i} \frac{W^{'}}{\exp(\frac{c (j+1)}{\mu}+p)+W^{'}} \cdot \frac{1}{\mu^i}}+
           p()
\end{equation}
\QEDA
%%%% New Section
%%%%%%%%%%%%%%%%%%%%%%%%%%%%%%%%%%
%%%%%%%%%%%%%%%%%%%%%%%%%%%%%%%%%%
%%%%%%%%%%%%%%%%%%%%%%%%%%%%%%%%%%
%%%%%%%%%%%%%%%%%%%%%%%%%%%%%%%%%%
